# Supplementary material for: Self-assembly of the discrete Sierpinski carpet and related fractals
Source: arXiv:0901.3189 source file (2009-01-21)
Supplement: Supplementary file 1 [file carpetmodp_appendix.tex]

%
% NOTE: This is a fragment of the complete LaTeX document carpetmodp.tex
%

Let $\LL$ be a finite alphabet and $n > 0$. Given an infinite two-dimensional
matrix $M: \mathbb{Z}^2 \rightarrow \LL$ and $x, y \in \mathbb{Z}$,
let $R_M(x,y)$ represent the $n-1 \times n$ submatrix
whose upper right corner is at $(x-1, y)$.  Formally, we think
of $R_M(x,y)$ as an element of $(\LL^n)^{n-1}$,
\[
R_M(x,y) = [\vec{r}_1, \vec{r}_2, \ldots, \vec{r}_{n-1}]^T,
\]
where each row vector $\vec{r}_i$ is defined as
\[
\vec{r}_i = (M[x-i, y-n+1], \ldots, M[x-i, y-1], M[x-i,y])
\]
for $1 \leq i < n$.
Let $\vec{r}_M(x,y)$ denote the vector consisting
of the $n-1$ elements of row $x$ directly to the
left of $(x,y)$, i.e.,
\[
\vec{r}_M(x,y) = (M[x, y-n+1], \ldots, M[x,y - 1]).
\]

Given a function $f$ defined on $\LL^{n^2 - 1}$, it will
be convenient to regard $f$ as a function on the domain
\[
\DD = {\LL_{\bot}}^{n-1} \times ({\LL_{\bot}}^n)^{n-1}.
\]
We will use symbols $\vec{q}, \vec{r}, \vec{s}$ for elements of 
${\LL_{\bot}}^{n-1}$ and $Q, R, S$ for elements of 
$({\LL_{\bot}}^n)^{n-1}$, so an element of the domain of 
$f$ can be written $(\vec{r}, R)$.

Let $\vec{N}$, $\vec{S}$, $\vec{E}$, $\vec{W}$ denote the four 
directional unit vectors in $\mathbb{Z}^2$.  

\begin{theorem}
Let $\LL$ be any finite alphabet and let $\bot$ be a symbol not in $\LL$.
Let $\LL_{\bot} = \LL \cup \{\bot\}$.  Let $f$ be any function
\[
f: {\LL_{\bot}}^{n^2 - 1} \rightarrow \LL.
\]
Define the infinite, two-dimensional matrix $M : \mathbb{Z}^2 \rightarrow \LL$
by 
\begin{eqnarray*}
M[x,y] &=& \bot \mbox{\ if $x < 0$ or $y < 0$} \\
M[x,y] &=& f(\vec{r}_M(x,y), R_M(x,y)) \mbox{\ otherwise.}
\end{eqnarray*}
Then there is a directed tile assembly system $\TT = (T, \sigma, 2)$, and
a labeling $m:T \rightarrow \LL$, such that in the unique terminal assembly
$\alpha$ of \ $\TT$, $m(\alpha(x,y)) = M(x,y)$ for all $x,y \geq 0$.
\end{theorem}

\begin{proof}
For each element
$(\vec{r}, R) \in \DD$, we define a tile type $t$.
Let 
\begin{eqnarray*}
\vec{r} &=& (r_0, r_1, \ldots, r_{n-2}), \\
R &=& [\vec{r}_1, \vec{r}_2, \ldots, \vec{r}_{n-1}]^T,\\
\end{eqnarray*}
and define
\begin{eqnarray*}
b &=& f(\vec{r}, R), \\
\vec{r'} &=& (r_1, r_2, \ldots, r_{n - 2}, b), \\
\vec{r}_0 &=& (r_0, r_1, \ldots, r_{n-2}, b), \mbox{\ and}\\ 
R' &=& [\vec{r}_0, \vec{r}_1, \vec{r}_2, \ldots, \vec{r}_{n-2}]^T.
\end{eqnarray*}
Then the color of $t = t(\vec{r}, R)$ is defined by
\begin{eqnarray*}
\mbox{col}_t(\vec{W}) &=& \vec{r} \\
\mbox{col}_t(\vec{S}) &=& R \\
\mbox{col}_t(\vec{E}) &=& \vec{r'} \\
\mbox{col}_t(\vec{N}) &=& R' \\
\end{eqnarray*}
and tile $t$ is labeled as $m(t) = b$.
\begin{center}
%left, bottom, right, top, center
\tile{$\vec{r}$}{$R$}{$\vec{r'}$}{$R'$}{$b$}
\end{center}

The strength of $t$ is $\mbox{str}_t(\vec{u}) = 1$ for all unit
vectors $\vec{u}$ except for the following cases:
\begin{description}
\item[Seed tile: ]
If $\vec{r}_i = (\bot, \ldots, \bot)$ for $1 \leq i < n$ and $\vec{r} = (\bot, \ldots, \bot)$, 
then $\mbox{str}_t(\vec{N}) = 2$ and $\mbox{str}_t(\vec{E}) = 2$.
\item[Row 0:]
If $\vec{r}_i = (\bot, \ldots, \bot)$ for $1 \leq i < n$ but $\vec{r} \neq (\bot, \ldots, \bot)$, 
then $\mbox{str}_t(\vec{W}) = 2$ and $\mbox{str}_t(\vec{E}) = 2$.
\item[Column 0:]
If $\vec{r}_i = (\bot, \bot, \ldots, \bot, r)$, where $r \neq \bot$, for $1 \leq i < n$ and
$\vec{r} = (\bot, \ldots, \bot)$,
then $\mbox{str}_t(\vec{S}) = 2$ and $\mbox{str}_t(\vec{N}) = 2$.
\end{description}
Define the seed assembly for $\TT$ by $\sigma(0,0) = s$, where $s$ is 
the unique seed tile described above.

It is not difficult to show that there exists a $2$-$T$-assembly sequence whose terminal
assembly has domain $\mathbb{Z}^+ \times \mathbb{Z}^+$, and that the
terminal assembly is unique.

Let $\{\alpha_i\}_{i \geq 0}$ be any $2$-$T$-assembly sequence.  Wlog
we assume that $\{\alpha_i\}_{i \geq 0}$ is a single-tile assembly
sequence, so that $|\mbox{dom}(\alpha_i)| = i$.   
We will show the following by induction on $i$:
\begin{enumerate.alph}
\item
For all $x,y \in \mbox{dom}(\alpha_i)$, $\alpha_i(x', y')$ 
is defined for all $0 \leq x' \leq x$ and $0 \leq y' \leq y$.
\item 
If $x < 0$ or $y < 0$, $\alpha_i(x,y)$ is undefined.  
\item
If $t = \alpha_i(x, y)$ has $\mbox{str}_t(\vec{E}) = 2$, then
$x = 0$
\item
If $t = \alpha_i(x, y)$ has $\mbox{str}_t(\vec{N}) = 2$, then
$y = 0$
\item
For all $x,y \in \mbox{dom}(\alpha_i)$, $\alpha(x,y)$ 
is the tile $t = t(\vec{r}, R)$ where $\vec{r} = \vec{r}_M(x,y)$
and $R = R_M(x,y)$.

\end{enumerate.alph}

Clearly (a)--(e) hold for the seed assembly 
$\sigma = \alpha_0$.  Let $i \geq 0$ and
let $(x,y)$ be the unique element of $\mbox{dom}(\alpha_{i+1})$ that 
is not in $\mbox{dom}(\alpha_i)$.  Let $t = \alpha_{i+1}(x,y)$.  By (a), 
$\alpha_i(x, y + 1)$ and $\alpha_i(x + 1, y)$ are undefined. 

{\em Case 1: \ } If $x > 0$ and $y > 0$, let 
\begin{eqnarray*}
t_{\rm left} &=& \alpha_i(x, y - 1) \mbox{\ and} \\
t_{\rm below} &=& \alpha_i(x - 1, y).
\end{eqnarray*}
By (c) and (d), both of $t_{\rm left}$ and $t_{\rm below}$ are
defined and 
$\mbox{str}_{t_{\rm left}}(\vec{E}) = \mbox{str}_{t_{\rm below}}(\vec{N}) = 1$.
Let
\begin{eqnarray*}
\vec{s} &=& \mbox{col}_{t_{\rm left}}(\vec{W}), \\
S &=& \mbox{col}_{t_{\rm left}}(\vec{S}), \\
\vec{s'} &=& \mbox{col}_{t_{\rm left}}(\vec{E}), \\
S' &=& \mbox{col}_{t_{\rm left}}(\vec{N}), \\
\end{eqnarray*}
and
\begin{eqnarray*}
\vec{q} &=& \mbox{col}_{t_{\rm below}}(\vec{W}), \\
Q &=& \mbox{col}_{t_{\rm below}}(\vec{S}), \\
\vec{q'} &=& \mbox{col}_{t_{\rm below}}(\vec{E}), \\
Q' &=& \mbox{col}_{t_{\rm below}}(\vec{N}) \\
\end{eqnarray*}
By (e), we know that
\begin{eqnarray*}
\vec{s} &=& \vec{r}_M(x,y-1), \\ 
S &=& R_M(x,y-1), \\
\vec{q} &=& \vec{r}_M(x-1,y), \mbox{\ and}\\ 
Q &=& R_M(x-1,y).
\end{eqnarray*}
Let $a = f(\vec{s}, S)$ and $c = f(\vec{q}, Q)$.  By 
the definition of $M$, $a = M[x,y-1]$ and $c = M[x-1, y]$.
Then by construction, $Q' = R_M(x,y)$ and
$\vec{s'} = \vec{r}_M(x,y)$.  
It follows that
\begin{eqnarray*}
\mbox{col}_t(\vec{W}) &=& \vec{r}_M(x,y) \mbox{\ and} \\
\mbox{col}_t(\vec{S}) &=& R_M(x,y), 
\end{eqnarray*}
establishing (e).

{\em Case 2:\ } If $x = 0$, $\alpha_i(x - 1, y)$ is undefined
by (b).  Hence $\alpha(x, y -1) = t'$ for some tile $t'$ with
$\mbox{str}_{t'}(\vec{E}) = 2$.

{\em TODO...}

{\em Case 3:\ } If $y = 0$, $\alpha_i(x, y - 1)$ is undefined
by (b).  Hence $\alpha(x, y -1) = t'$ for some tile $t'$ with
$\mbox{str}_{t'}(\vec{N}) = 2$.

{\em TODO...}

\end{proof}
